# Supplementary material for: HyperJump: Accelerating HyperBand via Risk Modelling
Source: arXiv:2108.02479 source file (2022-12-02)
Supplement: Supplementary file 1 [file supple_hyperjump_aaai23.pdf]

# Supplementary Material for HyperJump: Accelerating HyperBand via Risk Modelling

**Pedro Mendes[1,2], Maria Casimiro[1,2], Paolo Romano[2], David Garlan[1]**

[1] Software and Societal Systems Department, Carnegie Mellon University
[2] INESC-ID and Instituto Superior Técnico, Universidade de Lisboa
{pgmendes, mdaloura, dg4d}@andrew.cmu.edu, romano@inesc-id.pt

This document provides additional details about different aspects of HyperJump (HJ), a novel hyper-parameter optimization method that builds upon HyperBand's (HB) robust search strategy and accelerates it via an innovative, model-based technique. Specifically, this document is organized as follows:

- **Section 1** presents a visual overview of HyperJump's search process.
- **Section 2** provides details about the custom GP kernel employed by HyperJump to predict the quality of untested configurations.
- **Section 3** discusses how the equations for computing the Expected Accuracy Reduction (EAR) can be mathematically derived and numerically computed.
- **Section 4** provides details on the heuristic employed to select the candidate sets of configurations for a jump.
- **Section 5** details the pseudo-code for the heuristic used to select the next configurations to evaluate in a stage.
- **Section 6** details additional mechanisms exploited in HJ to speed up the optimization process.
- **Section 7** overviews the computational complexity of HJ.
- **Section 8** details the benchmarks used to evaluate HJ.
- **Section 9** discusses the implementation of the software used to evaluate HyperJump and provides information on how it can be obtained.
- **Section 10** presents additional experimental results comparing HJ to several state-of-the-art approaches.
- **Section 11** extends the ablation study of HyperJump to additional benchmarks.
- **Section 12** presents a study that evaluates the impact of tuning the risk threshold $\lambda$ on HJ's performance.
- **Section 13** evaluates the benefits of the strategy for bracket warm starting used in HyperJump.
- **Section 14** evaluates the reliability of the proposed risk modelling techniques (i.e., the rEAR).

## 1 Overview of HyperJump's search process

In this section, we present a visual representation of HyperJump's search process and compare it to HyperBand's (Li et al. 2018). Figure 1 aims to show the underlying mechanisms of HJ that allow it to find optimal configurations faster than HB. In the figure, we assume that both approaches start at time $T0$ considering the same set of configurations to be explored [1]. Additionally, we can see that HJ keeps track of the risk of jumping, which is initially very high given that the models have no knowledge about the quality of any configuration. Since the risk of jumping is too high (higher than the jumping threshold – depicted by the red line above the slider), HyperJump continues testing configurations in the current stage (i.e., no jumps are performed). While HB selects the next configuration to explore at random, HJ employs a heuristic that aims to maximize the reduction of the risk in order to favor earlier jumps. As such, while HB explores configuration $C1$, HJ explores configuration $C4$. By incorporating the knowledge acquired after testing $C4$ into the GP model, the risk of jumping decreases. At time $T5$, i.e., after testing 5 configurations, the risk of jumping decreases below the threshold for HJ, thus leading to a jump. The target stage to jump to and the set of configurations to include in the jump are computed based on the heuristic detailed in Section 3.1 of the paper.

In the example of Figure 1, HJ skips stage 1 completely and includes in the target stage of the jump (i.e., stage 2) configurations $C5$ and $C3$. Note here that, when determining which configurations to include in the stage targeted by a jump, HJ may select configurations that were still unexplored in the current stage, such as $C3$ in this example. The intuition for this behavior is detailed in Section 3.1 of the main body of the paper and in Section 4 of the supplemental material. At time instant $T6$, HJ is already in stage 2 while HB keeps on exploring configurations in stage 0. At time $T7$, HJ has evaluated configuration $C5$. As the risk of jumping drops below the threshold, the exploration of configuration $C3$ is skipped and HJ moves to the next stage with configuration $C5$. At time $T8$, HB completes stage 0 and HJ is already in the last stage of the first bracket. By the time HB begins stage 1, i.e. time $T9$, HJ has already found a new incumbent, configuration $C5$. Note that the identification of a new incumbent triggers also an update of the risk threshold, which causes HJ to adapt its future behavior and become,

Copyright © 2023, Association for the Advancement of Artificial Intelligence (www.aaai.org). All rights reserved.

[1] Note that HJ includes the bracket warm-starting technique, which is not considered in this example.

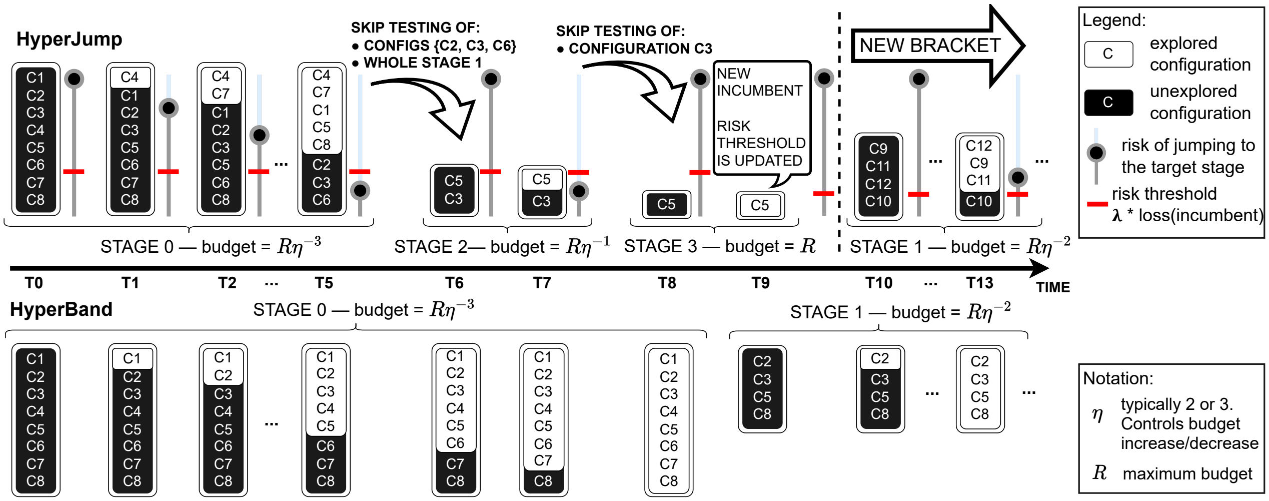


Figure 1: Comparison of the search methodologies of HJ (top) and HB (bottom). While HB randomly selects configurations to explore, HJ is guided by a heuristic that aims to select the next configuration such that the risk of jumping is minimized. This is depicted in the figure through the different set of configurations explored by each approach. Additionally, since the risk threshold is computed based on the loss of the incumbent, whenever HJ finds a new incumbent, the risk threshold is updated. This is depicted at time $T9$.

over time, progressively less risk-prone. Finally, HJ begins a new bracket at time $T10$ while HB is still exploring configurations in stage 1 and has not yet identified an incumbent (as no full budget configurations have been tested yet).

## 2 Models used to predict the quality of untested configurations

This section provides additional details on the models used by HJ to predict the quality of untested configurations. As already mentioned, in our implementation of HJ we opted for GPs as underlying black-box modelling toolkit, as GPs are among the most popular modelling technique used in the literature of BO (Brochu, Cora, and de Freitas 2010; Snoek, Larochelle, and P. Adams 2012; Lam, Willcox, and Wolpert 2016). Note that, in principle, alternative modelling techniques could be exploited (e.g., an ensemble of GPs (Breiman 1996, 2001) or Adaptive Bayesian linear regression (Valkov et al. 2018)) provided that they can not only predict the mean value but also estimate the predictions' uncertainty via a Gaussian distribution.

Similarly to recent related works (Klein et al. 2017, 2020; Mendes et al. 2020), we include in the feature space of the GP models not only the hyper-parameters' space, but also the budget (so as to enable inter-budget extrapolation). Further, analogously to, e.g., (Klein et al. 2017; Mendes et al. 2020), we employ a custom Bayesian Linear Kernel that encodes the expectation that the loss function has an exponential decay with larger budgets, along with a generic Matérn 5/2 kernel (Matérn 1986) that is used to capture relations among the hyper-parameters. More in detail, we normalized each dimension of the search space, and decided to model the loss (instead of accuracy). Thus, all the dimensions associated to the hyper-parameters to be optimized use the Matérn 5/2 kernel. The basis function used to capture variations of the budget is instead defined as:

$$\phi(b^*) = (1, (1-b^*)^2)^T \tag{1}$$

Note that we normalized each dimension, thus $b^* \in [0, 1]$.

Finally, also similarly to prior work, e.g., (Falkner, Klein, and Hutter 2018), we start using the model (and enable HJ's jumping logic) only after having gathered at least $d$+2 observations, where $d$ is the number of dimensions of the search space.

## 3 Computing the Expected Accuracy Reduction

This section provides details on how to compute the Expected Accuracy Reduction (EAR). Recall that the EAR of a jump from stage $s$ to stage $s+1$ in which we discard the configurations in $\mathcal{D}$ and select the ones in $\mathcal{S}$ is defined as:

$$\begin{aligned} EAR_s^{s+1}(\mathcal{D},\mathcal{S}) &= \int_{-\infty}^{+\infty} P\left(\mathcal{A}_s^{\mathcal{D}} - \mathcal{A}_s^{\mathcal{S}} = x\right) \max\{\mathcal{A}_s^{\mathcal{D}} - \mathcal{A}_s^{\mathcal{S}}, 0\} dx \\ &= \int_{0}^{+\infty} xP\left(\mathcal{A}_s^{\mathcal{D}} - \mathcal{A}_s^{\mathcal{S}} = x\right) dx \end{aligned} \tag{2}$$

where we have noted with $\mathcal{A}_s^{\mathcal{D}} = \max_{c \in \mathcal{D}} A(c, b_s)$, $\mathcal{A}_s^{\mathcal{S}} = \max_{c \in \mathcal{S}} A(c, b_s)$, and $A(c, b_s)$ is the accuracy of configuration $c$ on budget $b_s = b\eta^s$. Before discussing how to compute Eq. (2), let us detail how to compute the probability distribution function (PDF) of $\mathcal{A}_s^{\mathcal{D}}$ and $\mathcal{A}_s^{\mathcal{S}}$.

Let $\mathcal{T}$ be an arbitrary subset of the configurations in stage $s$. We use the notation $\phi_{\mathcal{A}_s^{\mathcal{T}}}(x)$ and $\Phi_{\mathcal{A}_s^{\mathcal{T}}}(x)$ to refer to the PDF and CDF, respectively, of $\mathcal{A}_s^{\mathcal{T}}$. We distinguish three cases: (1) $\mathcal{T}$ contains only tested configurations that have

been evaluated via noise-free measurements; (2) $\mathcal{T}$ contains only untested configurations or configurations tested via noisy measurements; (3) $\mathcal{T}$ contains some configurations tested via noise-free measurements and configurations that are either untested or tested via noisy measurements

Let us start by considering the first case, i.e., $\mathcal{T}$ only contains configurations tested via noise-free measurements, such that all configurations in $\mathcal{T}$ are described by a Dirac $\delta$ function. In this case, the PDF of $\mathcal{A}_s^{\mathcal{T}}$ is simply:

$$\phi_{\mathcal{A}_s^{\mathcal{T}}}(x) = \delta(x - \max_{c\in\mathcal{T}} A(c, b_s)) \tag{3}$$

If $\mathcal{T}$ only contains untested configurations or if the tested configurations are subject to noisy measurements, then the accuracy predictions for any configuration in $\mathcal{T}$ follow a normal distribution. The CDF of $\mathcal{A}_s^{\mathcal{T}}$, noted $\Phi_{\mathcal{A}_s^{\mathcal{T}}}$, can then be computed in closed form as the product of the CDFs of the normal distributions associated with the configurations $c \in \mathcal{T}$, i.e., $\Phi_{A(c,b_s)}$:

$$\Phi_{\mathcal{A}_s^{\mathcal{T}}}(x) = \prod_{c\in\mathcal{T}} \Phi_{A(c,b_s)}(x) = \prod_{c\in\mathcal{T}} \Phi\left(\frac{x-\mu_{A(c,b_s)}}{\sigma_{A(c,b_s)}}\right) = \exp\left(\sum_{c\in\mathcal{T}} \log \Phi\left(\frac{x-\mu_{A(c,b_s)}}{\sigma_{A(c,b_s)}}\right)\right), \tag{4}$$

where we have denoted with $\Phi(x)$ the CDF of the standard normal distribution and with $\mu_{A(c,b_s)}$, $\sigma_{A(c,b_s)}$ the average and standard deviation of the predicted accuracy of $c$ with budget $b_s$, respectively. Then, we can determine the PDF by computing the derivative of the CDF:

$$\phi_{\mathcal{A}_s^{\mathcal{T}}}(x) = \frac{d}{dx}\Phi_{\mathcal{A}_s^{\mathcal{T}}}(x) = \prod_{c\in\mathcal{T}} \Phi\left(\frac{x-\mu_{A(c,b_s)}}{\sigma_{A(c,b_s)}}\right) \cdot \sum_{c\in\mathcal{T}} \frac{\phi\left(\frac{x-\mu_{A(c,b_s)}}{\sigma_{A(c,b_s)}}\right)}{\sigma_{A(c,b_s)}\Phi\left(\frac{x-\mu_{A(c,b_s)}}{\sigma_{A(c,b_s)}}\right)} \tag{5}$$

where $\phi(x)$ is the PDF of the standard normal distribution.

Finally, let us consider the case in which $\mathcal{T}$ contains both configurations associated with Gaussian distributions (i.e., untested configurations or tested via noisy measurements) and configurations associated with Dirac $\delta$ functions (i.e., tested via noise-free measurements). Let us denote with $\mathcal{T}_\delta$ and $\mathcal{T}_\mathcal{N}$ the former and latter subset of configurations of $\mathcal{T}$, respectively. The PDF of $\mathcal{A}_s^{\mathcal{T}}$ is then given by

$$\phi_{\mathcal{A}_s^{\mathcal{T}}}(x) = H(x - \max_{c\in\mathcal{T}_\delta} A(c, b_s)) \frac{\phi_{\mathcal{A}_s^{\mathcal{T}_\mathcal{N}}}(x)}{P_{\mathcal{A}_s^{\mathcal{T}_\mathcal{N}}}(x \geq \max_{c\in\mathcal{T}_\delta} A(c, b_s))} \tag{6}$$

where $H$ is the Heaviside function and $\phi_{\mathcal{A}_s^{\mathcal{T}_\mathcal{N}}}(x)$ can be computed using Eq. (5).

Let us now discuss how to compute Eq. (2). The distribution $Z = \mathcal{A}_s^{\mathcal{D}} - \mathcal{A}_s^{\mathcal{S}} = X + Y$ can be computed as the convolution between two random variables $X$ and $Y$.

$$f_Z(x) = f_X(x) * f_Y(y) = \int_{-\infty}^{+\infty} f_X(k) f_Y(x-k) dk. \tag{7}$$

Hence, Eq. (2) can be computed as:

$$EAR_s^{s+1}(\mathcal{D}, \mathcal{S}) = \int_0^{+\infty} \int_{-\infty}^{+\infty} f_X(k) f_Y(k-x) x \, dk \, dx, \tag{8}$$

where $f_X$ and $f_Y$ are obtained by Eq. (5). As an optimization, we take advantage of the existence of tested configurations with noise-free measurements (i.e., associated with Dirac $\delta$ functions) in $\mathcal{S}$ and/or $\mathcal{D}$ to simplify Eq. (8).

If all the configurations in $\mathcal{S}$ are associated with a Dirac $\delta$ function and the configurations in $\mathcal{D}$ are all associated with normal distributions, then Eq. (2) can be rewritten as:

$$EAR_s^{s+1}(\mathcal{D}, \mathcal{S}) = \int_0^{+\infty} [f_X(x) * f_Y(x)] x \, dx = \int_0^{+\infty} f_X(x + \max_{c_i\in\mathcal{S}} A(c_i, b_s)) x \, dx, \tag{9}$$

where $f_Y$ is given by Eq. (3) and $f_X(x)$ by Eq. (5).

Analogously, if all the configurations in $\mathcal{D}$ are tested and modelled by a Dirac $\delta$ function (i.e., $f_X$ is determined using Eq. (3)) and $\mathcal{S}$ contains only configurations associated with normal distributions (i.e., $f_Y(x)$ is determined using Eq. (5)), the EAR can be computed as:

$$EAR_s^{s+1}(\mathcal{D}, \mathcal{S}) = \int_0^{+\infty} f_Y(-x + \max_{c\in\mathcal{D}} A(c, b_s)) x \, dx \tag{10}$$

Finally, in case only some (but not all) of the configurations in $\mathcal{D}$ or $\mathcal{S}$ are associated with a Dirac $\delta$ function, Eq. (8) can be simplified by reducing the interval of integration of the convolution due to the computation of the Heaviside function. For example, if both sets have tested and untested configurations, the EAR can be simplified by

$$EAR_s^{s+1}(\mathcal{D}, \mathcal{S}) = \int_0^{+\infty} \int_M^{+\infty} \frac{\phi_{\mathcal{A}_s^{\mathcal{D}_\mathcal{N}}}(k)}{P_{\mathcal{A}_s^{\mathcal{D}_\mathcal{N}}}(k \geq \max_{c_i\in\mathcal{D}_\delta} A(c_i, b_s))} \cdot \frac{\phi_{\mathcal{A}_s^{\mathcal{S}_\mathcal{N}}}(k-x)}{P_{\mathcal{A}_s^{\mathcal{S}_\mathcal{N}}}(k - x \geq \max_{c_i\in\mathcal{S}_\delta} A(c_i, b_s))} x \, dk \, dx \tag{11}$$

where $M = \max\{\max_{c\in\mathcal{D}_\delta} A(c, b_s); x + \max_{c\in\mathcal{S}_\delta} A(c, b_s)\}$. It should be noted that despite the presence of the double max in the equation above, a regular integral can be used. This is because the inner max operators in the definition of $M$ are constant values (representing the accuracy of the best tested configuration in the set of discarded and selected configurations, respectively), so they can be simplified

Finally, note that, although the PDF and the CDF of $X$ and $Y$ are known in closed form, the convolution can not be computed analytically (and, as such, neither can Eq. (2)). Therefore, we need to resort to numerical methods to compute the convolution and determine the distribution $Z$ and the respective expected value. Those were implemented in Python3.6 using the function *nquad* of the *scipy* package. Moreover, for efficiency reasons, we implemented in C the function to integrate that is called via the *LowLevelCallable* function. We use the default configuration values of *nquad*,

Algorithm 1: Pseudo-code of the mechanism used to select the next configuration to test in a stage (function NEXT_CONF_TO_TEST()).

Set⟨Config,risk⟩ NEXT_CONF_TO_TEST(Set⟨Config⟩ Untested, Set⟨Config⟩ Tested, int $s$)
Set⟨Config,risk⟩ C=∅
**for** $x$ ∈ Untested **do**
    ▷ *Use GP model to predict accuracy of an untested configuration $x$,*
    $acc$ = model.predictedAccuracy($x$,$b\eta^s$)
    T$^*$ = Tested ∪ $\{\langle x, acc\rangle\}$; U$^*$ = Untested \ $\{x\}$
    ▷ *Estimate the risk of jumping after emulating testing $x$ via the model*
    risk = EVALUATE_JUMP_RISK($s$, T$^*$, U$^*$).getJumpRisk()
    $C = C \cup < x$, risk $>$
**end for**
▷ *Return the (untested) configuration with minimum estimated risk*
**return** $x$ s.t. $\langle x$,risk$\rangle \in C \wedge \forall \langle y$,risk$'\rangle \in C$ : risk$' \geq$ risk

except for the absolute error tolerance (which we set to $1^{-12}$) and the upper bound on the number of sub-intervals used in the adaptive algorithm (which we set to 2500).

## 4 Determining the candidate sets of configurations targeted by a jump

In this section, we provide additional details on the logic used by HJ to determine the sets of configurations to be considered when jumping from stage $s$ to stage $s+1$. This logic was already informally described in Section 3.1 and is used by Algorithm 2 (in the main body of the paper) where it is encapsulated into the function GET_CANDIDATES_FOR_$\mathcal{S}$. In order to further clarify the logic of this function we also exemplify its execution in Figure 2.

## 5 Selecting the next configurations to evaluate in a stage

Algorithm 1 reports the pseudo-code of the NEXT_CONF_TO_TEST() function, which is responsible for determining the next configuration to test in the current stage. The logic of this function was described in Section 3.2 of the main body of the paper.

## 6 Additional Optimizations

HJ adopts additional optimizations that aim, resp., at selecting promising configurations to evaluate in a new bracket — *bracket warm starting* —, reducing the cost of evaluating configurations that were previously tested with lower budgets — *pause-resume training* — and increasing, at no extra cost, the information that can be fed to the model — *opportunistic evaluation*.

**Selecting the configurations for a new bracket.** To further accelerate HB, HJ leverages BO to determine which configurations to include when a new bracket is started — an idea already exploited in prior work, e.g., (Falkner, Klein, and Hutter 2018; Wang, Xu, and Wang 2018; Bertrand et al. 2017) and also referred to as bracket warm starting. In more detail, HJ uses its models to identify which set of configurations maximizes the EI when deployed using *full budget* — recall that, as in HB, our aim is to maximize accuracy using the full budget. This allows HJ to leverage prior knowledge, unlike HB, at no considerable extra cost, since no additional models are trained nor maintained.

**Pause-resume training.** In a HB's bracket, configurations are tested multiple times with increasing budget values. HJ takes advantage of this observation by saving the model obtained after evaluating a configuration $c$ with budget $b^\dagger$, noted $\mathcal{M}(c, b^\dagger)$. If later on (in the same or in a different HJ bracket), $c$ is tested again with budget $b^* > b^\dagger$, HJ reloads $\mathcal{M}(c, b^\dagger)$ and resumes the training (thus reducing the "cost" of training by $b^\dagger$). Note that this optimization is not new in the context of hyper-parameter optimization, e.g., (Swersky, Snoek, and Adams 2014; Golovin et al. 2017; Liaw et al. 2018).

**Opportunistic evaluation.** In modern ML frameworks, (e.g., NNs trained using the parameter server approach (Li et al. 2014)), the model's validation error is typically monitored (and made available) throughout the training process and not only upon its conclusion. We take advantage of this as follows. Assume that a configuration $c$, so far not tested with budget $b^\dagger$, is requested to be tested with budget $b^* > b^\dagger$ (e.g., when HJ jumps from the first to the last stage). In such a case, during the evaluation of $c$ with budget $b^*$, when the training process reaches budget $b^\dagger$ we measure the model's current accuracy, noted $acc(c, b^\dagger)$ and extend the model's dataset with the observation $\langle c, b^\dagger, acc(c, b^\dagger)\rangle$, enriching its knowledge base in an *opportunistic* fashion, i.e., at no additional cost. A similar optimization was already introduced in the Raytune framework (Liaw et al. 2018).

## 7 Computational Complexity of HJ

This section presents an evaluation of the computational complexity of the main mechanisms of HJ. The main computational costs incurred by HJ are related to: i) evaluating whether to perform a jump and, if so, which configurations to include in the target stage, namely EVALUATE_JUMP_RISK() (see Alg. 3 in the main body of the paper), ii) determining which configuration to explore in the current stage if no jump is performed, namely NEXT_CONF_TO_TEST() (see Alg. 1 in the supplemental material), and iii) updating (i.e., training) the underlying (GP) model when new knowledge is available following the testing of a configuration .

Let us start by evaluate the complexity of the EVALUATE_JUMP_RISK() function. To this end, we first need to determine the complexity of the GET_CANDIDATES_FOR_$\mathcal{S}$() function described in Algorithm 2 in the main body of the paper. This function first sorts the configurations by accuracy, LCB and UCB, which yields a complexity of $\mathcal{O}(|\mathcal{C}| \log |\mathcal{C}|)$. Next, as discussed in Section 3.1.2, it generates $1{+}2\lfloor \log_\eta |\mathcal{C}/\eta| \rfloor$ candidates for $\mathcal{S}$. Thus, the complexity of the GET_CANDIDATES_FOR_$\mathcal{S}$() function is $\mathcal{O}\left(|\mathcal{C}| \log |\mathcal{C}| + \log_\eta |\mathcal{C}|/\eta\right)$. Recall that the notation $|\mathcal{C}|$ refers to the number of configurations in the current stage, including both tested and untested ones.

The computation of the EAR for one candidate set requires initializing data structures (e.g., lists) having size $\mathcal{O}(|\mathcal{C}|)$ and computing via numerical methods the integral of

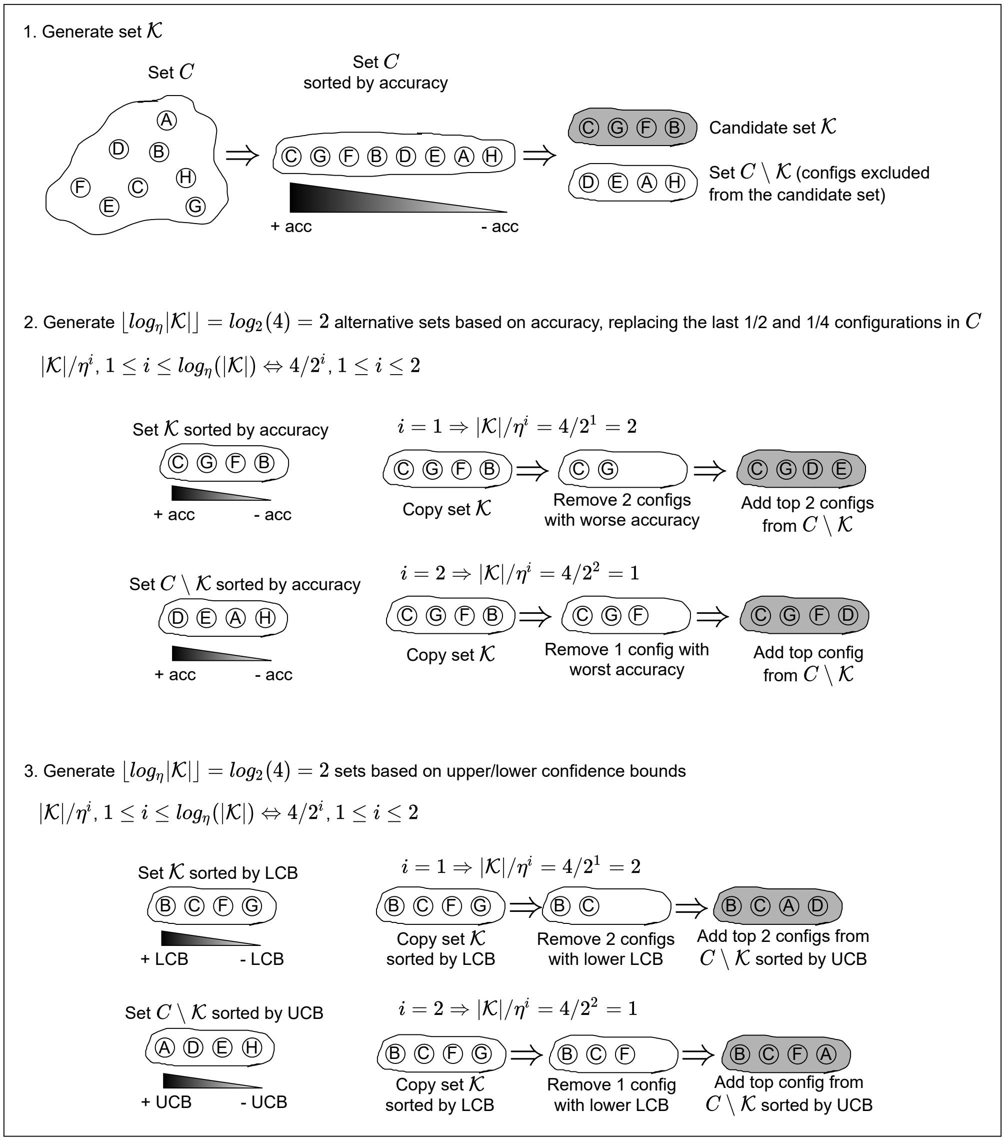


Figure 2: Illustration of the execution of the GET_CANDIDATES_FOR_$\mathcal{S}$ function, introduced in Section 3.1 of the main body of the paper. This function is used to determine the alternative sets of configurations to consider for a jump from stage $s$ to $s+1$. The alternative sets are highlighted in grey.

Eq. (2). In our implementation, we employ the *nquad* function of the *scipy* library that has complexity $\mathcal{O}(m^d)$ (Kong, Siauw, and Bayen 2020), where $d$ is the dimensionality of the integral and $m$ is the number of points/sub-intervals employed to approximate the integral. Given that the integral of Eq. (2) is over a single dimension (i.e., accuracy), overall we get complexity $\mathcal{O}(|\mathcal{C}| + m)$.

For a 1-hop jump, HJ evaluates the rEAR on 1+2$\lfloor \log_\eta |\mathcal{C}|/\eta \rfloor$ candidate sets. Thus, the complexity to find the best candidate set that minimizes the risk of 1-hop jumps is $\mathcal{O}\left((|\mathcal{C}| + m) \log_\eta |\mathcal{C}|/\eta\right)$.

Overall, the complexity of the EVALUATE_JUMP_RISK() function for 1-hop jumps is $\mathcal{O}\left(|\mathcal{C}| \log |\mathcal{C}| + (|\mathcal{C}| + m) \log_\eta |\mathcal{C}|/\eta\right)$. The complexity of EVALUATE_JUMP_RISK() function for a generic multi-hop jump, which in the worst case skips up to $S-1$ stages, is thus $\mathcal{O}\left(S|\mathcal{C}| \log |\mathcal{C}| + S(|\mathcal{C}| + m) \log_\eta |\mathcal{C}|/\eta\right)$, where $S$ is the number of stages per bracket.

Next, we evaluate the complexity of the NEXT_CONF_TO_TEST() function, whose pseudo-code is described in Algorithm 1 of the supplemental material. Since this function invokes EVALUATE_JUMP_RISK() to compute the risk for each untested configuration in the current stage ($U$), its complexity is simply $|U|$ times the complexity of EVALUATE_JUMP_RISK(). In the worst case, when all configurations are untested (i.e., $U = \mathcal{C}$), the complexity is $\mathcal{O}\left(S|\mathcal{C}|^2 \log |\mathcal{C}| + S|\mathcal{C}|(|\mathcal{C}| + m) \log_\eta |\mathcal{C}|/\eta\right)$.

At last, the complexity due to updating and retraining the

Table 1: SVM hyper-parameters.

| Parameter | Values |
|---|---|
| Kernel | {linear, polynomial deg. 2, polynomial deg. 3, polynomial deg. 4, RBF, Sigmoid} |
| Gamma | {1e-6,1e-5,1e-4,1e-3,5e-3,1e-2,5e-3,0.1,0.5,1, 2,5,7,10,20,30,40,50,60,70,80,90,100} |
| C | {1e-6,1e-5,1e-4,1e-3,5e-3,1e-2,5e-3,0.1,0.5,1, 2,5,7,10,20,30,40,50,60,70,80,90,100} |

models after evaluating a new configuration is dependent on the choice of the underlying modelling technique. Since in HJ, we employ GPs to predict configuration quality, the model re-retrain complexity is $\mathcal{O}(N^3)$ (Belyaev, Burnaev, and Kapushev 2014), where $N$ is the training set size (i.e., total number of configurations explored during the optimization process).

Overall, if $S$ and $\eta$ are considered as constants in the above analysis (typical values for these two variables are 5 and 3, respectively), HJ's complexity can be rewritten as $\mathcal{O}\left(|\mathcal{C}|(|\mathcal{C}| + m) \log |\mathcal{C}| + N^3\right)$.

## 8 Benchmarks

This section provides additional details on the benchmarks that we used to evaluate HyperJump. Firstly, we benchmark HJ using the NATS-Bench (Dong et al. 2021) data set, where we optimize the topology of the cells of a NN and fix to four the number of layers and the hyper-parameters (see (Dong et al. 2021; Dong and Yang 2020) for more details). This data set considers 5 different connection topologies (zeroize, skip connection, 1-by-1 convolution, 3-by-3 convolution, and 3-by-3 average pooling layer), and the search space encompasses 6 dimensions (each one represents a connection between two layers and have 5 possible topologies). This benchmark contains an exhaustive evaluation of all possible 15625 configurations and the accuracy and training time is evaluated in each epoch. Thus, in this case, we considered the number of epochs as budget and consider 200 epochs to be the largest possible/full budget.This benchmark provides data sets describing the model's quality for all possible hyper-parameter values when trained using: i) ImageNet-16-120 (Russakovsky et al. 2015), ii) Cifar100, and iii) Cifar10 (Krizhevsky and Hinton 2009).

Next, we considered the training of a Support Vector Machine (SVM) implemented via the LIBSVM (Chang and Lin 2011) framework and trained on the Covertype data set (Dua and Graff 2017). Due to time and hardware constraints, we reduced the data set size by $\approx 5\times$. In this case, we considered a smaller number of dimensions (i.e., 3 dimensions) but a higher number of configurations. The considered hyper-parameters are the kernel (linear, polynomial with degree from 2 to 4, RBF, and sigmoid), $\gamma$, and C, and the respective values are reported in Table 1. Note that in this case we could not exhaustively explore off-line the hyper-parameter space, so the optimum is unknown.

Furthermore, in this supplemental material, we provide more experiments to evaluate HJ using different models and

Table 2: Hyper- and cloud parameters.

| Parameter | Values |
|---|---|
| Learning rate | $\{10^{-3}, 10^{-4}, 10^{-5}\}$ |
| Batch size | $\{16, 256\}$ |
| Training mode | {sync, async} |

| VM type | VM characteristics | #VMs |
|---|---|---|
| t2.small | {1 vCPU, 2 GB} | {8,16,32,48,64,80} |
| t2.medium | {2 vCPU, 4 GB} | {4,8,16,24,32,40} |
| t2.xlarge | {4 vCPU, 16 GB} | {2,4,8,12,16,20} |
| t2.2xlarge | {8 vCPU, 32 GB} | {1,2,4,6,8,10} |

data sets. We also deployed in the AWS cloud the distributed training of 3 different neural networks (NNs): a Convolutional Neural Network (CNN), a Multilayer Perceptron (MLP), and a Recurrent Neural Network (RNN). We consider a parameter space composed of 6 dimensions: batch size, learning rate, and training mode (synchronous vs asynchronous[2]), as well as the number, type, and size of the virtual machines used for training. This space was discretized and the considered values are resumed in Table 2.

We trained the NNs using the MNIST data set (Deng 2012) with 60000 images to train and 10000 images to test the NN. We trained in each of the different configurations using 5 different sub-sampled data sets and also measured the model's validation loss periodically. We set an additional timeout to stop the training after 10 minutes in order to control and bound the cost to pay in the cloud. This is a common approach when training machine learning (ML) models in the cloud (Mendes et al. 2020; Casimiro et al. 2020).

We created a variant of the above benchmarks using the training time as budget, instead of data set size. This was done by considering as the full budget a 10 minutes training time; the intermediate time and accuracy values measured when training with the full data set were then used to derive the model's accuracy at intermediate (time) budgets. We also extended both data sets produced via these experiments in order to benchmark HJ in a neural architecture search (NAS) scenario, in which we also optimize the NN architecture (CNN, MLP, or RNN) by adding an dimension to the search space corresponding to the architecture to use.

Note that we included in the search space not only the model's hyper-parameters, but also the type and number of virtual machines employed, since, as shown in prior work, e.g., (Zhang et al. 2016; Casimiro et al. 2020), the size and characteristics of the underlying computing infrastructure can have a strong impact on the efficiency of the worker's synchronization and model convergence speed. More in detail, in both the above mentioned scenarios (data set size or training time as budget) we rely on a parameter server archi-

[2]Note that this hyper-parameter controls how the training phase is parallelized, i.e., whether the parameter server waits for all the workers to send in their updates before updating the model or not (Li et al. 2014). This hyper-parameter is not to be confused with the notion of synchronous vs asynchronous parallelization of HB, as defined by (Li et al. 2020).

Table 3: UNET hyper- and hardware parameters.

| Parameter | Values |
|---|---|
| Learning rate | $\{10^{-4}, 10^{-5}, 10^{-6}\}$ |
| Batch size | $\{1, 2\}$ |
| Momentum | $\{0.9, 0.95, 0.99\}$ |
| Training mode | {sync, async} |
| **GPU type** | **#GPUs** |
| GeForce GTX 1080 | $\{1, 2\}$ |
| GeForce RTX 2080 Super | $\{1, 2\}$ |

tecture to train the NNs, either in a synchronous or asynchronous mode. In these settings the choice of the number of workers, once we fix the model's hyper-parameters (in particular synchronous vs asynchronous training), can have a large impact on accuracy. In particular, when setting training time as budget, using more powerful machines intuitively yields higher accuracy with the same budget and hyper-parameter settings. As for the case of using data set size as budget, we have experimentally observed that the model's accuracy varies significantly if we change the number and type of VMs over which we train the model, even using the same hyper-parameters. For instance, using a large number of machines with small data sets and high learning rates can cause the training procedure to become unstable (after an initial improvement, validation loss tends to degrade over time), whereas the model built using a single worker achieves a much higher accuracy.

At last, we considered Light UNET (Ronneberger, Fischer, and Brox 2015) (trained with the 2017 CCF BDCI data set). Also in this case the search space is composed of 6 dimensions/hyper-parameters (see Table 3): batch size, learning rate, momentum, training mode, as well as the type and number of GPUs installed on the machine used for training. In this case we also discretized the search space and exhaustively sampled it by training the model in each configuration during 5 hours and measuring its accuracy periodically.

In all the benchmarks described so far (except for NATS-Bench), in order to reduce noise in the measurements, we trained each configuration three times, monitoring the model's accuracy periodically, and considered the average of these runs. To test HJ in a broader range of settings, we consider two different values of the $\eta$ parameter (2 for CNN, NAS, UNET, NATS-Bench with Cifar10; 3 for the others) and different budgets (we use time as budget in RNN, MLP and UNET; number of epochs in NATS-Bench; and training set size for the remaining benchmarks).

## 9 Software

HyperJump was implemented based on the publicly available code of BOHB (Falkner, Klein, and Hutter 2018). Moreover, we used this implementation to deploy BOHB and HB. ASHA was implemented via the Ray-Tune (Liaw et al. 2018) framework, while to evaluate Fabolas, we used its publicly available implementation provided by the authors. We also implemented a version using BO with EI and Random Search. All the optimizers were implemented in Python 3.6 and deployed on VMs equipped with 16 vCPUs and 16GB of RAM; the underlying cloud compute nodes are equipped with two AMD EPYC 7501 CPUs.

We have made available the implementation of HJ[3] and the benchmarks used [4]. In order to ensure reproducibility of results, the source code already includes scripts to generate the same random seeds and reproduce the results presented in this work. We also provide instructions on how to use the scripts.

## 10 Additional results comparing HJ with state-of-the-art optimizers

This section presents supplementary data regarding the comparison of HJ with respect to the set of baseline optimizers described in Section 4 of the submitted manuscript.

Figure 3 reports the average loss as a function of the wall clock time (i.e., training and recommendation time) for all the benchmarks used to evaluate HJ in a sequential deployment scenario (1 worker). Note that in this figure we are including additional results that we had to omit from the main body of the paper due to space constraints. In order to ease visualization and comparison among benchmarks, we include in Figure 3 also the benchmarks that were already presented in Figure 2 of our submission.

In all the benchmarks, HJ provides significant speed-ups with respect to all the baselines to identify both configurations of good quality as well as near optimal ones. The largest speed-ups for recommending good quality solutions are achieved in CNN, UNET, NATS-Bench, NAS, and RNN, where the gains of HJ w.r.t. the best baseline range from around 20$\times$ to 10$\times$. As for identifying close to optimum configurations, the largest speed-ups against the best baseline are achieved in NATS-Bench using Cifar100 and ImageNet ($\approx$21$\times$ and $\approx$19$\times$), RNN and MLP ($\approx$10$\times$ in both benchmarks), CNN and NAS ($\approx$5$\times$ in both) and UNET ($\approx$2.5$\times$).

It can be noted that for some benchmarks, e.g., UNET and NAS MNIST, HyperJump's result show a relatively larger variance when compared to other baselines. This is due to the fact that in some runs, HyperJump jumps earlier than in other runs, which leads to increasing variance especially in the early stages of the run. In other words, differently from solutions, like BOHB and HB, which follow a very regular exploration policies (strictly dictated by successive halving), HyperJump is, by design, more prone to adapt its exploration policy depending on the model perceived risk, which leads to a relatively larger variance.

Moreover, we report in Table 4 (i) the total number of configurations evaluated by each optimizer at the time corresponding to the maximum value in the x-axis plots in Figure 3 and (ii) the total search space for each benchmark, including the different possible "budgets" (namely 5). We observe that HJ evaluates less configuration than similar multi-

[3] https://github.com/pedrogbmendes/HyperJump

[4] https://drive.google.com/drive/folders/18FwyVbZHJSALkwaUceB6iXz4BmX5FmqZ?usp=sharing

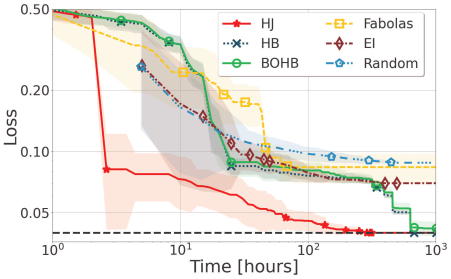


(a) UNET (1 worker)

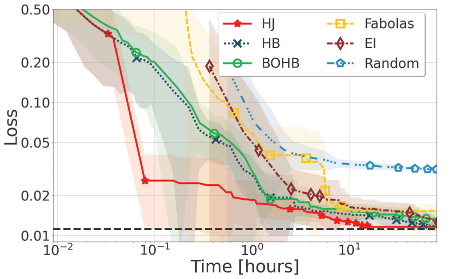


(b) CNN MNIST (1 worker)

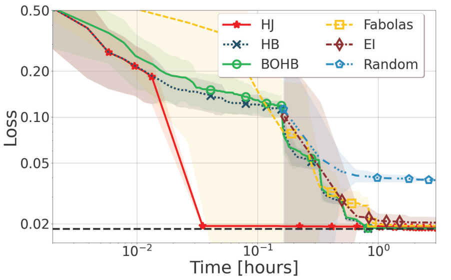


(c) RNN MNIST(1 worker)

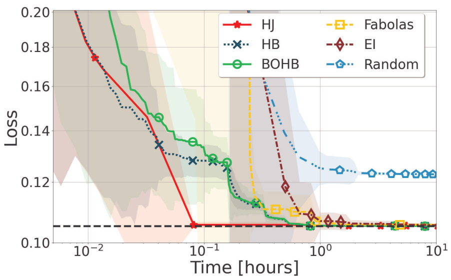


(d) MLP MNIST (1 worker)

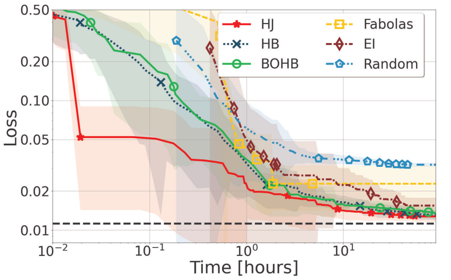


(e) NAS MNIST (1 worker)

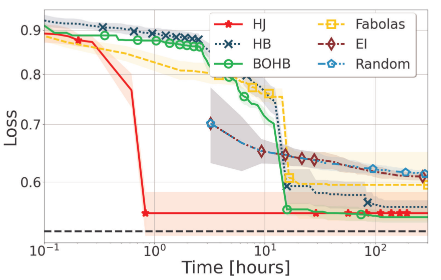


(f) NATS-Bench ImageNet (1 worker)

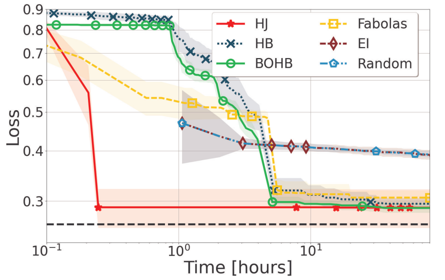


(g) NATS-Bench Cifar100 (1 worker)

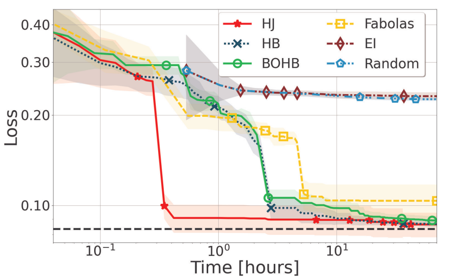


(h) NATS-Bench Cifar10 (1 worker)

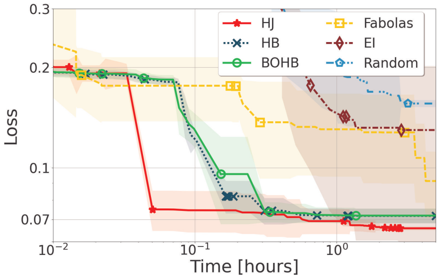


(i) SVM Covertype (1 worker)

Figure 3: Comparison of HJ against other state-of-the-art optimizers in a sequential deployment scenario (1 worker).

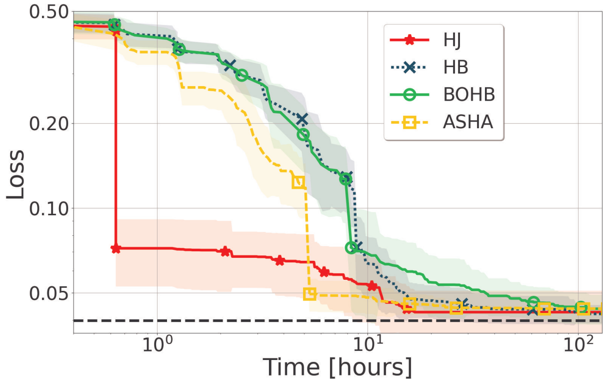


(a) UNET (8 workers)

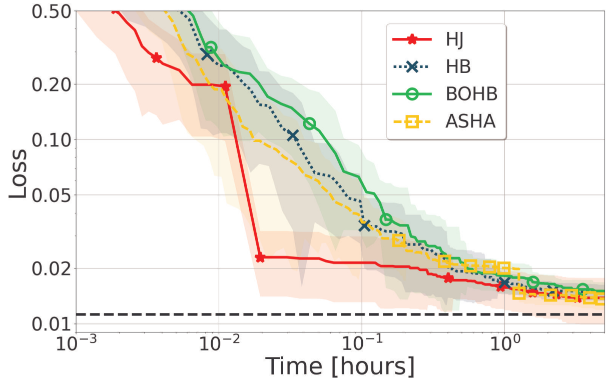


(b) CNN MNIST(8 workers)

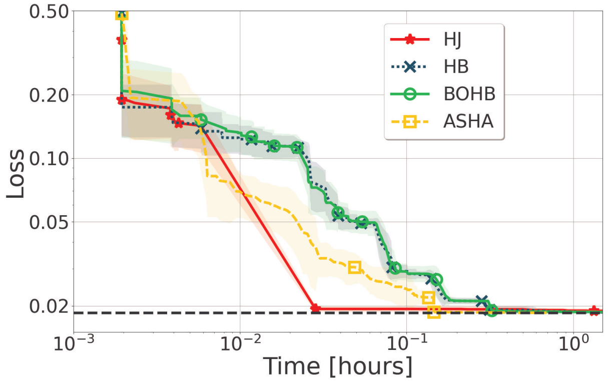


(c) RNN MNIST (8 workers)

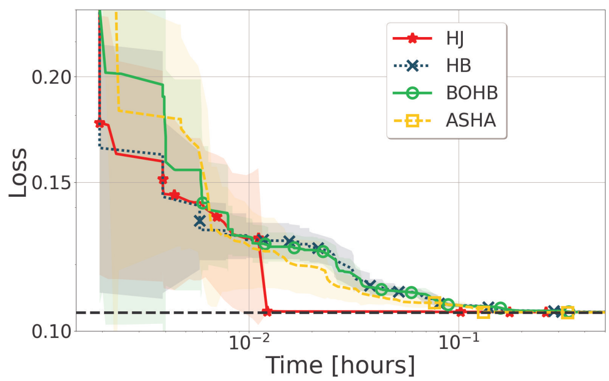


(d) MLP MNIST (8 workers)

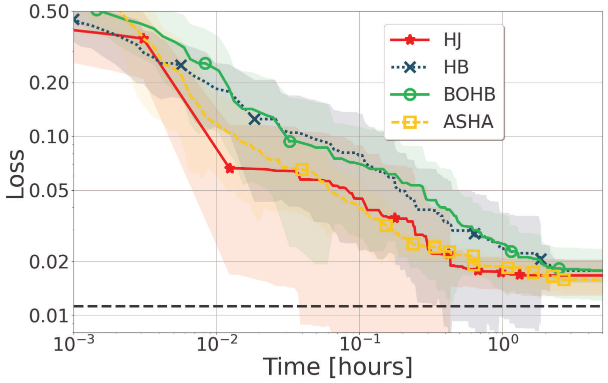


(e) NAS MNIST(8 workers)

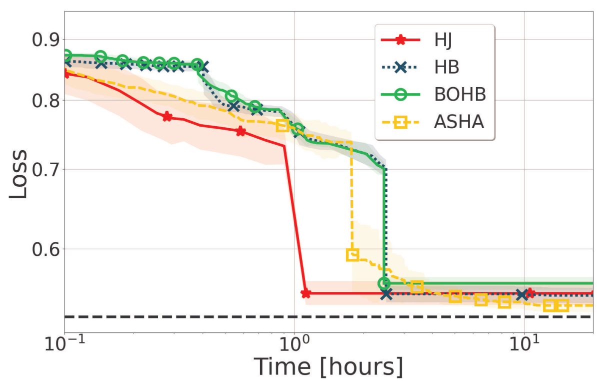


(f) NATS-Bench ImageNet (8 workers)

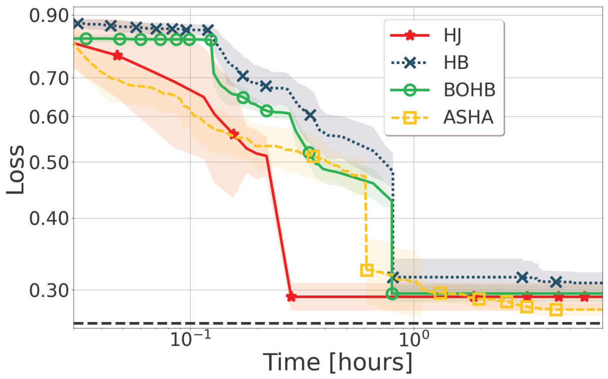


(g) NATS-Bench Cifar100 (8 worker)

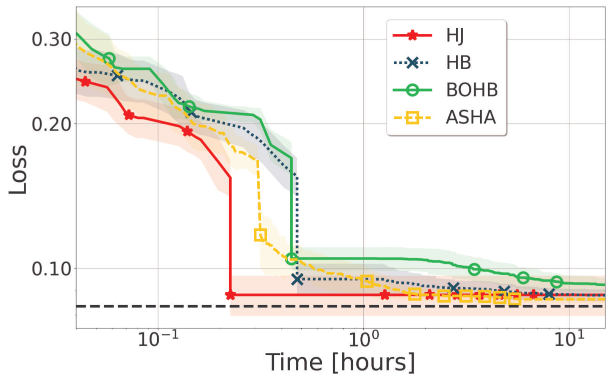


(h) NATS-Bench Cifar10 (8 workers)

Figure 4: Comparison of HJ against other state-of-the-art optimizers in a parallel deployment scenario using 8 workers.

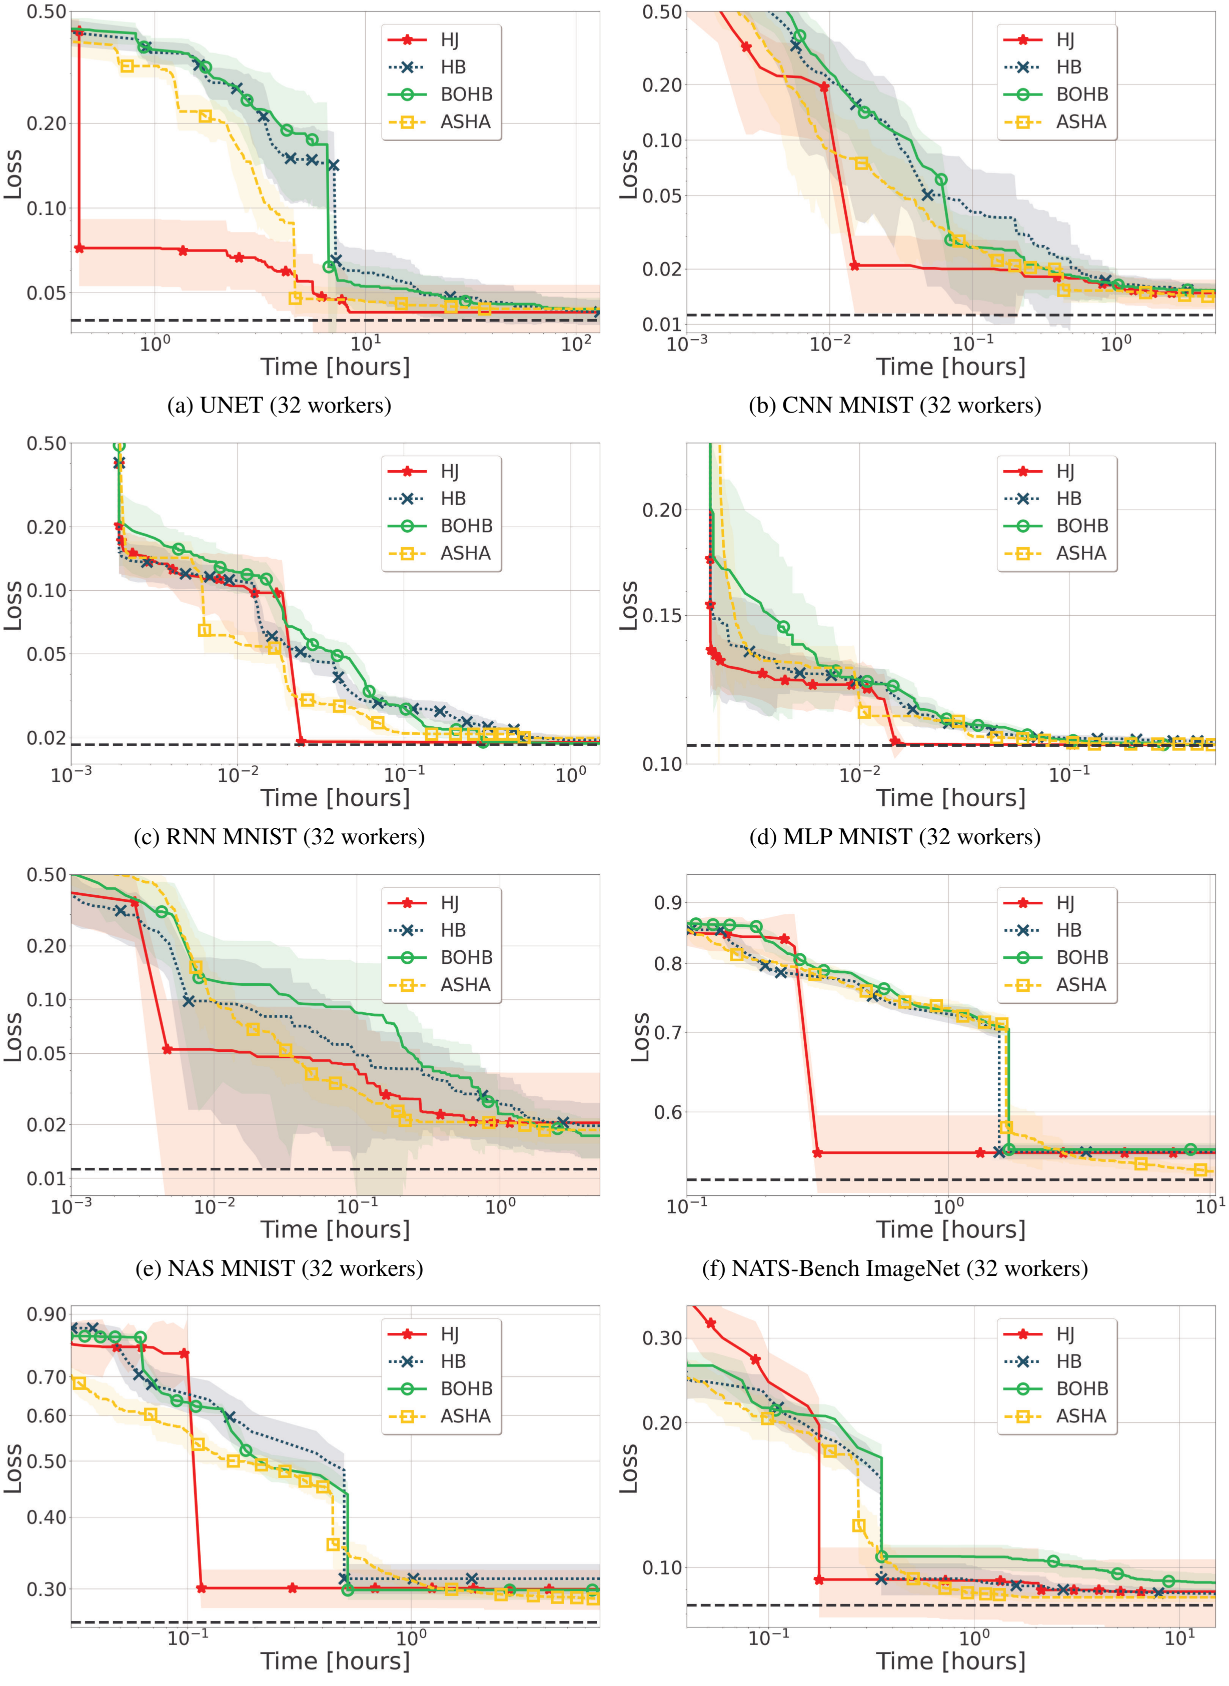


(a) UNET (32 workers)
(b) CNN MNIST (32 workers)
(c) RNN MNIST (32 workers)
(d) MLP MNIST (32 workers)
(e) NAS MNIST (32 workers)
(f) NATS-Bench ImageNet (32 workers)
(g) NATS-Bench Cifar100 (32 workers)
(h) NATS-Bench Cifar10 (32 workers)

Figure 5: Comparison of HJ against other state-of-the-art optimizers in a parallel deployment scenario using 32 workers.

Table 4: Number of configurations tested

| | HJ | HB | BOHB | Fabolas | EI | search space size |
|---|---|---|---|---|---|---|
| **NATS cifar10** | 490 | 430 | 464 | 212 | 144 | 78125 |
| **NATS cifar100** | 518 | 738 | 992 | 175 | 76 | 78125 |
| **NATS imageNet** | 558 | 1196 | 1304 | 132 | 90 | 78125 |
| **Unet** | 300 | 330 | 424 | 72 | 204 | 500 |
| **CNN mnist** | 612 | 1028 | 1080 | 96 | 152 | 1440 |
| **RNN mnist** | 128 | 324 | 328 | 108 | 90 | 1440 |
| **MLP mnist** | 322 | 684 | 701 | 166 | 60 | 1440 |
| **NAS mnist** | 721 | 1340 | 876 | 74 | 374 | 4320 |
| **SVM covertype** | 522 | 845 | 740 | 150 | 72 | 15870 |

fidelity methods (i.e., HB and BOHB). We conclude that although HJ evaluates less number of configurations (due to the jumping mechanism that allow bypass the testing of configurations) and thus reduces the optimization time, it recommends better quality incumbents than HB and BOHB. Furthermore, as expected EI evaluates less but expensive configurations.

In Figure 4 and Figure 5, we report the results for the scenario of parallel deployments with 8 and 32 workers for all the considered benchmarks except SVM, which we could not test due to resource constraints. In this case, we report again the data for the experiments of the benchmarks already included in Figure 1 of the main body of the paper, in order to ease visualization and comparison among benchmarks.

Let us start by analyzing the data in Figure 5 for the benchmarks which were not reported in the main body of the paper in the scenario of 32 workers. By analyzing the results obtained for these benchmarks and comparing them to the sequential case, we observe a slight reduction of the gains achieved by HJ in the early stage of the optimization with respect to the considered baselines (in particular compared to ASHA that aims at solving the parallelization drawbacks imposed by HB). Despite HJ's gains w.r.t. ASHA being slightly reduced, it is worth to highlight that HJ still achieves speed-ups of up to approximately 10× to recommend near-optimal configurations. In the less favourable scenarios for HJ (namely, NAS and MLP with MNIST), HJ achieves a performance comparable to ASHA, while still reducing the optimization time when compared to HB and BOHB. A possible explanation for this is that, when using $w$ number of parallel workers, the first $w$ configurations tested by HJ coincide necessarily with the first $w$ configurations tested by HB — recall that since we assume no a priori knowledge, we cannot instantiate a model at the start of the optimization process (see Section 2) and HJ samples configurations uniformly at random, just like HB. As such, as the number of workers increases, the performance gains of HJ in the early stage of the optimization (and in particular in the first stage/bracket) tend to get closer to those of HB. Nonetheless, it is worth highlighting that also with MLP, HJ achieves approximately one order of magnitude speed-ups to identify configurations that are close to optimum with respect to HB with respect to all considered baselines.

Finally, the plots in Figure 4 show, as expected, trends similar to the ones already analyzed in Figure 3 and Figure 5. This is expected, considering that the scenario considered in Figure 4, i.e., 8 workers, represents a middle ground with respect to the scenarios of 1 and 32 workers, analyzed in Figure 3 and Figure 5, respectively.

## 11 Ablation Study

In this section, we conduct an ablation study (see Figure 6) aimed at quantifying the contributions of the various mechanisms employed by HJ. The figure reports the performance achieved on NATS-Bench with ImageNet, Cifar100, and Cifar10, and UNET by four HJ variants obtained by disabling each of the following mechanisms: **(i)** the pause-resume training and opportunistic evaluation optimizations (HJ-no-Opt); **(ii)** the bracket warm-starting (HJ-no-BW); **(iii)** prioritizing the evaluation order of configurations (HJ-no-Ord); and **(iv)** the jumping logic (HJ-no-Jump). We include in the plot also HB, which can be regarded as a variant of HJ from which we disabled all of the mechanisms proposed in this paper. This data shows that the first three of these mechanisms have a similar impact on the performance of HJ. Using UNET (Figure 6a), disabling these mechanisms increases the time required by HJ to identify the optimum by nearly 40%; a similar slow-down factor can be observed also throughout the optimization process, e.g., the time taken to reach a loss of 5% is around 40% larger with HJ-no-Opt and around 80% larger with HJ-no-BW and HJ-no-Ord. Regarding ImageNet and Cifar100, we can see that disabling these optimizations lead to a relatively small degradation of the configuration that is finally recommended by HJ. For the case of Cifar100, we can also observe that disabling the pause-resume training and opportunistic evaluation optimizations can impose a slow down also throughout the optimization process.

Finally, and most importantly, in all these benchmarks, we can clearly see that the largest performance penalty is observed when disabling jumping. This confirms that this mechanism is indeed the one that contributes the most to HJ's efficiency.

## 12 Setting the Risk Threshold ($\lambda$)

This section reports the result of an experimental study that aimed to assess the sensitivity of HJ's performance to the setting of the risk threshold $\lambda$. We recall that $\lambda$ is the threshold that HJ uses to decide whether to consider a jump as

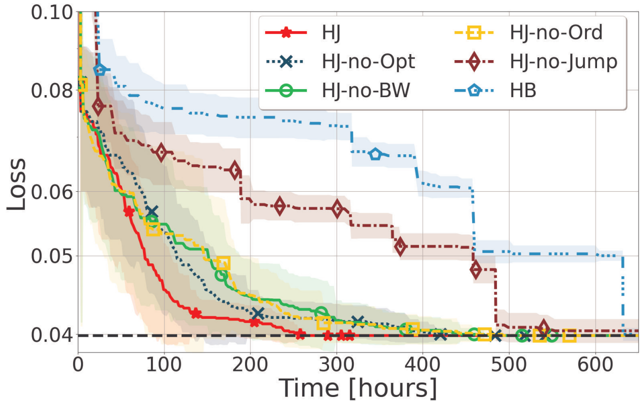


(a) UNET (1 worker)

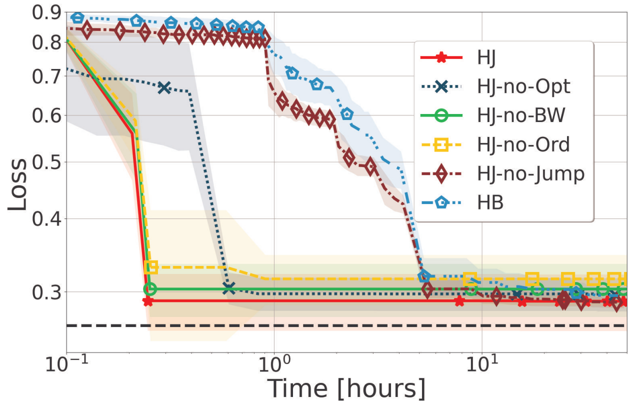


(b) NATS-Bench Cifar100 (1 worker)

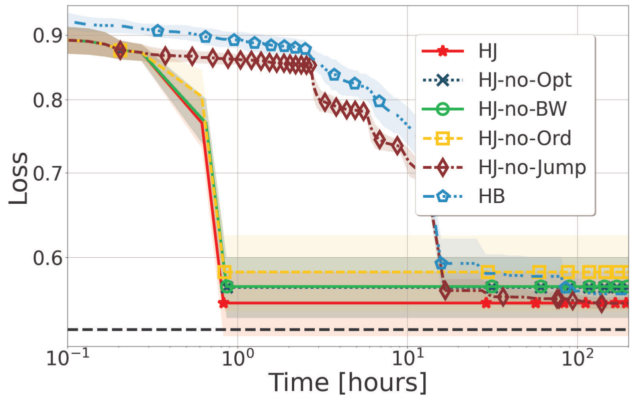


(c) NATS-Bench ImageNet (1 worker)

Figure 6: Ablation study in which we disable selectively the main mechanisms integrated in HJ. The results confirm that HJ's jumping mechanism is the one that contributes the most to the speed-ups that HJ achieves with respect to HB.

safe and that 0.1 is its recommended setting. To this end, we tested HJ on the same set of benchmarks (except SVM and NATS-Bench, for which we could not conduct this study due to resource and time constraints) using the following threshold values ($\lambda = \{10^{-3}, 10^{-2}, 10^{-1}, 1\}$) and report the corresponding results in Figure 7.

The key conclusion that can be drawn by analyzing these plots is that the performance of HJ does not vary significantly for values of $\lambda$ in the [$10^{-1}$,1] range, with the best overall performance being achieved when using $\lambda = 10^{-1}$.

We can also observe that the use of the smallest considered threshold settings, i.e., $10^{-2}$ and $10^{-3}$, has a negative impact on the convergence speed of HJ especially in the early stages of the optimization process. At the beginning of the optimization, in fact, models have relatively few available data. As a consequence, models have also higher uncertainty and larger threshold values need to be employed to allow HJ to shortcut HB's search procedure. The effects are particularly noticeable with MLP and RNN, where the use of larger threshold settings ($10^{-1}$ and 1) allows HJ to shortcut almost all of the intermediate stages of the first bracket and to jump to the last (i.e., the full-budget) stage and identify near-optimal configurations. This phenomenon is clearly visible in Figure 8, which reports, at the granularity of each stage, the distribution, average and median of the number of stages skipped by HJ for the runs when HJ does jump, considering different threshold settings. The data in Figure 8 was produced using the CNN data set, but analogous trends can be observed also in the other benchmarks.

By analyzing the data in Figure 8, we can also observe that in the first bracket HJ tends to perform longer jumps (i.e., skipping a larger number of stages) than in later brackets. This is due to the fact that HJ uses a risk metric (i.e., rEAR, see Section 3.1 of the main body of the paper) that is normalized by the loss of the current incumbent. As such, since in the first stage of the first bracket no incumbent is known yet (and its loss is assumed to be large, i.e., 1), the risk propensity of HJ is higher than in later brackets (when we have already identified an incumbent with smaller loss).

It is however worth noting that even in the later stages of the optimization process, HJ continues to avoid the testing of a significant fraction of the configurations prescribed by HB's logic — which is key to ensure HJ's competitiveness throughout the optimization process. Figure 9 provides a clear experimental support for this claim by reporting the distribution, average and median of the percentage of con-

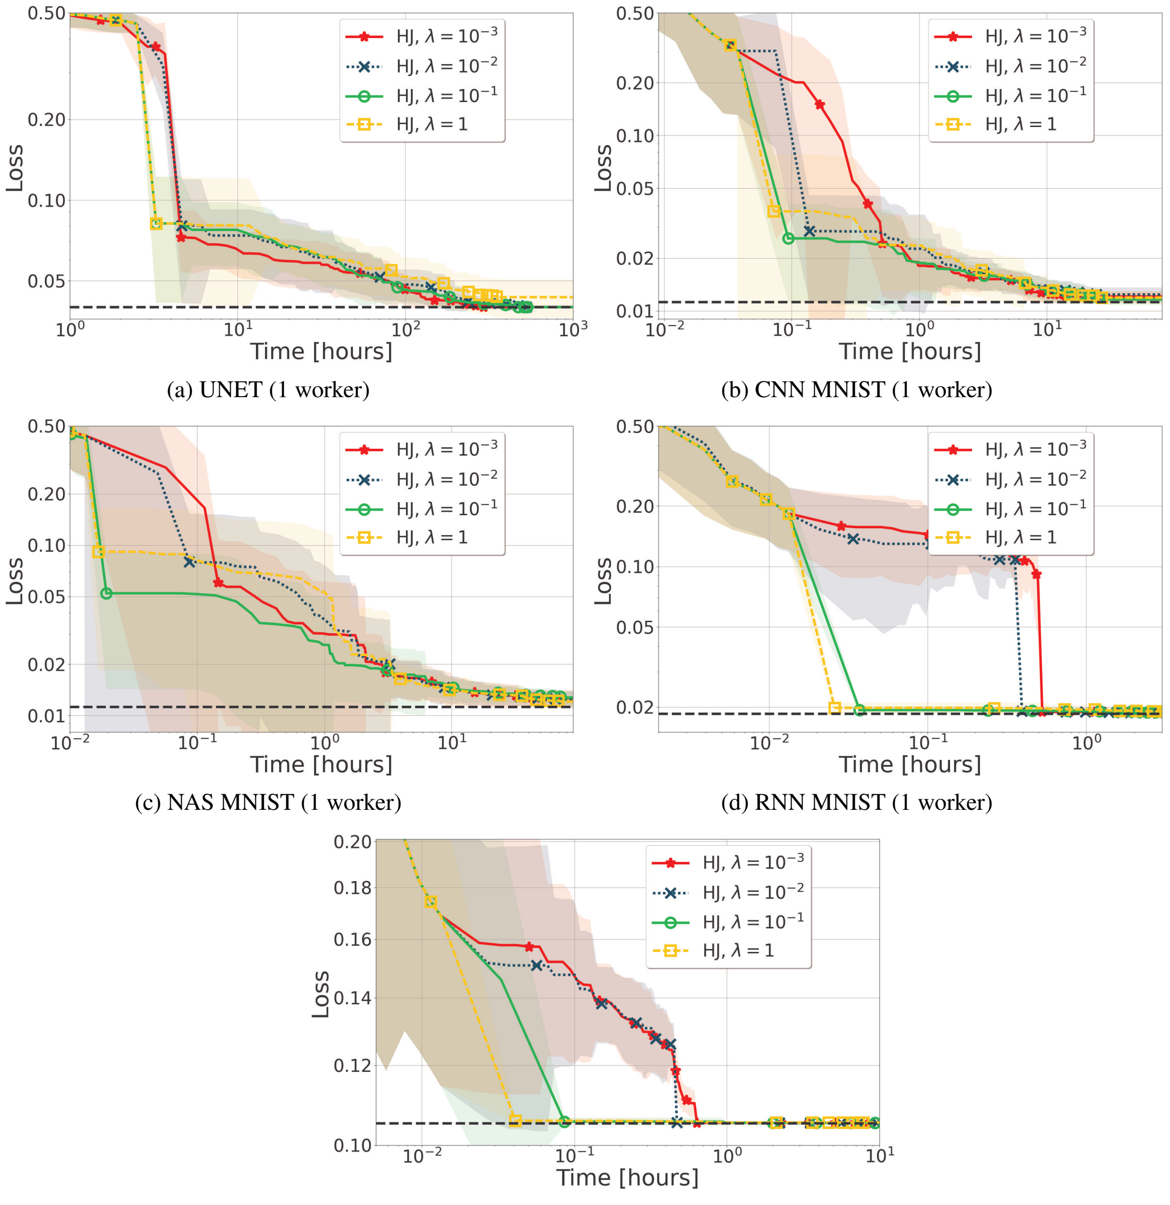


(a) UNET (1 worker) (b) CNN MNIST (1 worker) (c) NAS MNIST (1 worker) (d) RNN MNIST (1 worker) (e) MLP MNIST (1 worker)

Figure 7: Performance of HyperJump when using different thresholds values across several benchmarks.

figurations tested by HJ relative to the number of configurations tested by HB. Note that in Figure 9, we report data at the granularity of brackets in order to allow the visualization of an additional iteration of HJ and evaluate HJ's performance over a longer time scale. As expected, the largest reduction in the percentage of tested configurations is achieved in the first iteration and, in particular, in its first bracket (approx. 50% and 60% on average, respectively, when $\lambda$=0.1). However, also in the later stages of the optimization process, namely in the second and third iteration, HJ still allows for skipping the testing of approximately 35% of the configurations on average when using $\lambda = 0.1$ and approximately half of the configurations in brackets, e.g., 6, 9 and 11.

Overall, in light of this experimental data and for the benchmarks considered in this study, we can conclude that:

1. HJ provides robust performances in a relatively large range of settings for $\lambda$ (i.e., $\lambda \in [10^{-1}, 1]$ .
2. Setting $\lambda$ below $10^{-1}$ tends to reduce the effectiveness of HJ by forcing it to adopt overly conservative policies.

## 13 Bracket Warm Starting

This sections aims to evaluate the benefits stemming from using the proposed model-based methodology to warm start a new bracket (i.e., selecting the configurations to be included in a new bracket).

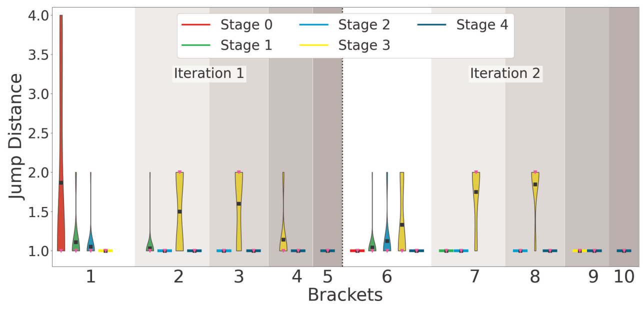


(a) $\lambda = 0.001$

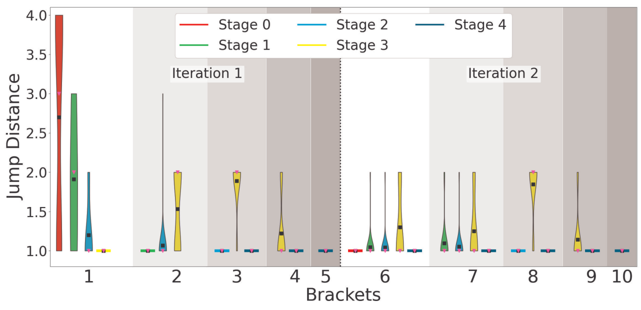


(b) $\lambda = 0.01$

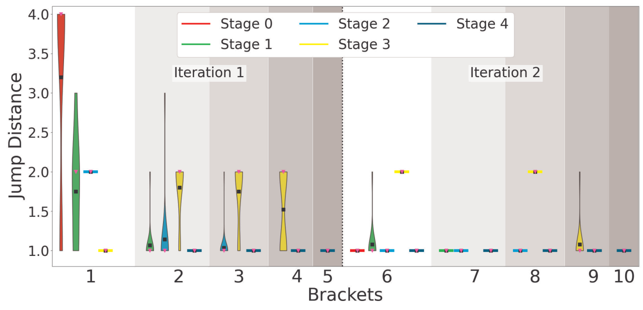


(c) $\lambda = 0.1$

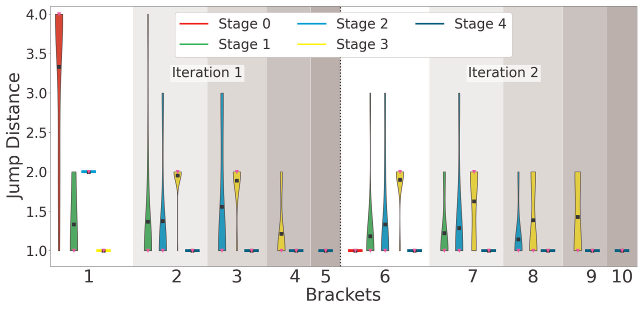


(d) $\lambda = 1.0$

Figure 8: Evaluation of the jump length per stage for the CNN benchmark. The violin plots depict the distribution of 30 independent runs, the respective average (black square), and median (pink triangle) value.

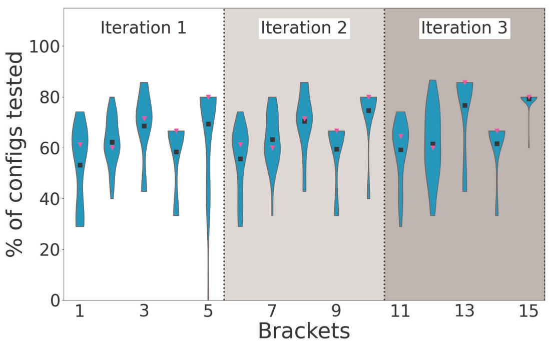


(a) $\lambda = 0.001$

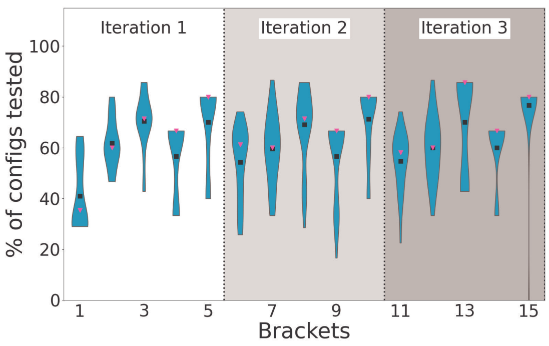


(b) $\lambda = 0.01$

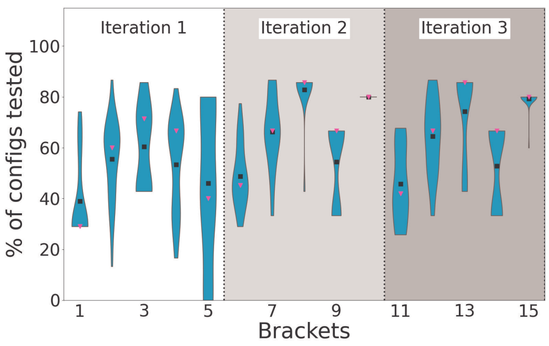


(c) $\lambda = 0.1$

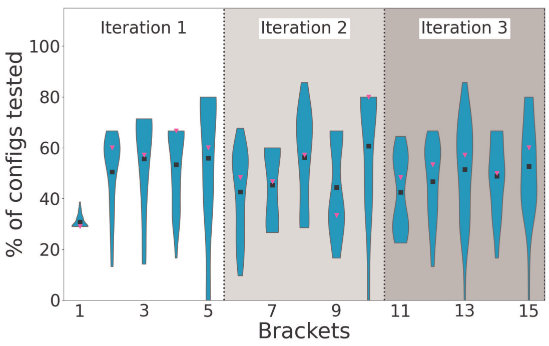


(d) $\lambda = 1.0$

Figure 9: Evaluation of the percentage of configurations tested by HJ with respect to HB at the granularity of stage for the CNN benchmark. The violin plots depict the distribution of 30 independent runs, the respective average (black square), and median (pink triangle) value.

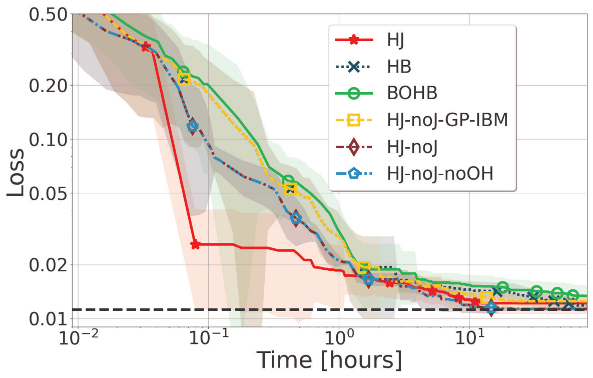


Figure 10: Comparison between different bracket warm starting techniques using CNN.

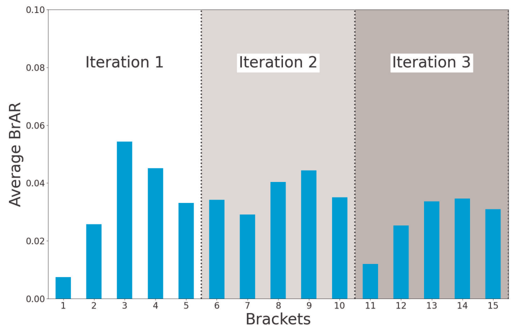


Figure 11: Average Real relative Accuracy Reduction (BrAR) due to a jump of the best configuration per bracket using CNN.

To this end, we report, in Figure 10, the results of an experimental study, based on CNN, in which we compare the following solutions:

- HB, which selects the configuration to include in a bracket uniformly at random.
- BOHB, which uses the Tree Parzen Estimator (TPE) to approximate EI and that employs an independent model per budget. Note that we use the official implementation of BOHB and its default settings. As such, 30% of the configurations are selected uniformly at random.
- A variant of HJ where we disable the jumping mechanism and that uses EI and GP as the base learner and employs an independent model per budget (similarly to BOHB). We refer to this baseline as HJ-noJ-GP-IBM in Figure 10.
- A variant similar to the previous one but instead it uses EI, GP as the base learner, and employs a single model that incorporates the budget among its features. We refer to this baseline as HJ-noJ in Figure 10.
- An "idealized" variant of HJ-noJ, referred to as HJ-noJ-noOH, in which we assume no overhead for recommending configurations for bracket warm starting (despite still using and training GP-based models).

Note that, in order to focus the study solely on the evaluation of different bracket warm starting techniques, we disabled HJ's jumping mechanism (by setting the risk threshold $\lambda$ to 0) both in the HJ-noJ and HJ-noJ-GP-IBM variants. Recall also that HJ, similarly to BOHB, samples 30% of the configurations uniformly at random to preserve the theoretical properties of HB. We preserve this behavior also in HJ-noJ and HJ-noJ-GP-IBM to ensure a fair comparison with BOHB.

By analyzing the plot, we see that HJ-noJ achieves approximately $8\times$ speed-ups to recommend the optimal configuration, as well as consistent speed-ups throughout the whole optimization process. By comparing HJ-noJ and HJ-noJ-GP-IBM, we can also observe that the key factor that contributes to HJ-noJ's superior performance is the adoption of a single model that incorporates the budget among its features. This can be concluded by observing that the performances of HP-noJ-GP-IBM and BOHB are very similar and recalling that the only difference between the two solutions is that the former uses EI, whereas the latter adopts TPE.

At last, the variant HJ-noJ-noOH can be seen as an ideal baseline that can deliver high quality recommendations by employing GPs — which as already discussed provides better quality predictions than, e.g., BOHB's TPE — without incurring any recommendation overhead. The analysis of this variant allows us to draw two main conclusions. First, even when compared with such an ideal variant, HJ preserves its large speed-ups. Second, since the performance of HJ-noJ-noOH and HJ-noJ (which does account for recommendation overhead) are essentially indistinguishable, we can conclude that, even with relatively small datasets (MNIST), the overhead of the proposed recommendation technique (based on GPs) is quite small.

## 14 Evaluating the predictions for the risk jumping

In this section, we evaluate the effectiveness of the proposed risk modelling technique, namely the rEAR, which HJ exploits to determine whether to skip the testing of configurations in the current stage. To this end, the plot in Figure 11 reports, for the CNN benchmark and a risk threshold of 10%, the average value of the real relative accuracy reduction of the best configuration obtained by HJ at the end of each bracket when compared to a variant of, HJ-no-jump, that includes all of HJ's mechanisms with the exception of jumps. We call this measure per-Bracket relative Accuracy Reduction (BrAR).

In more detail, the plot in Figure 11 reports the average of the BrAR over 30 runs, where, for each run, we execute both HJ and HJ-no-jump with the same random seeds, which ensures that at the configurations selected for testing in each bracket is the same for both variants. We then execute both variants till the end of a bracket and, denoting the best configuration at the end of the bracket for HJ and HJ-no-jump as $c^*_{HJ}$ and $c^*_{HJ-no-jump}$, respectively, we compute the BrAR

for that bracket as:

$$BrAR = \frac{c^*_{HJ-no-jump} - c^*_{HJ}}{l^*_{HJ}}$$

where $l^*_{HJ}$ is the incumbent's loss at the time in which the bracket starts for HJ.

The plot shows that the average BrAR is consistently below 10%, which corresponds to the risk threshold $\lambda$ that HJ uses to bound the rEAR for an individual jump. Note that the BrAR metric reflects the relative accuracy reduction due all the jumps that possibly take place within a bracket (i.e., possibly more than one jump). As such, the rEAR and BrAR are not directly comparable. Yet, the fact that the average BrAR is below $\lambda$ (i.e, 10%) implies that the rEAR is also below 10%. This confirms the effectiveness of the proposed risk modelling method — recall that HJ aims at ensuring that the expected value of the rEAR due to a single jump is lower than the risk threshold.

## References


Belyaev, M.; Burnaev, E.; and Kapushev, Y. 2014. Exact Inference for Gaussian Process Regression in case of Big Data with the Cartesian Product Structure. arXiv:1403.6573.

Bertrand, H.; Ardon, R.; Perrot, M.; and Bloch, I. 2017. Hyperparameter optimization of deep neural networks: combining Hperband with Bayesian model selection. In *Proceedings of Conférence sur l'Apprentissage Automatique*.

Breiman, L. 1996. Bagging Predictors. *Machine Learning*, 24(2).

Breiman, L. 2001. Random Forests. *Machine Learning*, 45(1).

Brochu, E.; Cora, V. M.; and de Freitas, N. 2010. A Tutorial on Bayesian Optimization of Expensive Cost Functions, with Application to Active User Modeling and Hierarchical Reinforcement Learning. Technical Report arXiv:1012.2599.

Casimiro, M.; Didona, D.; Romano, P.; Rodrigues, L.; Zwanepoel, W.; and Garlan, D. 2020. Lynceus: Cost-efficient Tuning and Provisioning of Data Analytic Jobs. In *Proceedings 20th IEEE International Conference on Distributed Computing Systems*.

Chang, C.-C.; and Lin, C.-J. 2011. LIBSVM: A Library for Support Vector Machines. *ACM Transactions on Intelligent Systems and Technology*, 2.

Deng, L. 2012. The MNIST database of handwritten digit images for machine learning research [Best of the Web]. In *IEEE Signal Processing Magazine*, volume 29. IEEE.

Dong, X.; Liu, L.; Musial, K.; and Gabrys, B. 2021. NATS-Bench: Benchmarking NAS Algorithms for Architecture Topology and Size. *IEEE Transactions on Pattern Analysis and Machine Intelligence (TPAMI)*. doi:10.1109/TPAMI.2021.3054824.

Dong, X.; and Yang, Y. 2020. NAS-Bench-201: Extending the Scope of Reproducible Neural Architecture Search. In *International Conference on Learning Representations (ICLR)*.

Dua, D.; and Graff, C. 2017. UCI Machine Learning Repository.

Falkner, S.; Klein, A.; and Hutter, F. 2018. BOHB: Robust and Efficient Hyperparameter Optimization at Scale. In *Proceedings of the 35th International Conference on Machine Learning*, volume 80.

Golovin, D.; Solnik, B.; Moitra, S.; Kochanski, G.; Karro, J.; and Sculley, D. 2017. Google Vizier: A Service for Black-Box Optimization. In *Proceedings of the 23rd ACM SIGKDD International Conference on Knowledge Discovery and Data Mining*.

Klein, A.; Falkner, S.; Bartels, S.; Hennig, P.; and Hutter, F. 2017. Fast Bayesian Optimization of Machine Learning Hyperparamaters on Large Datasets. In *Proceedings of the 20th International Conference on Artificial Intelligence and Statistics*, volume 54.

Klein, A.; Tiao, L. C.; Lienart, T.; Archambeau, C.; and Seeger, M. 2020. Model-based asynchronous hyperparameter and neural architecture search. *arXiv preprint arXiv:2003.10865*.

Kong, Q.; Siauw, T.; and Bayen, A. 2020. *Python Programming And Numerical Methods: A Guide For Engineers And Scientists*. Elsevier.

Krizhevsky, A.; and Hinton, G. 2009. Learning multiple layers of features from tiny images. Technical report, University of Toronto.

Lam, R. R.; Willcox, K. E.; and Wolpert, D. H. 2016. Bayesian Optimization with a Finite Budget: An Approximate Dynamic Programming Approach. In *Proceedings of the 29th Neural Information Processing Systems Conference*.

Li, L.; Jamieson, K.; DeSalvo, G.; Rostamizadeh, A.; and Talwalkar, A. 2018. Hyperband: A novel bandit-based approach to hyperparameter optimization. *Journal of Machine Learning Research*, 18: 1–52.

Li, L.; Jamieson, K.; Rostamizadeh, A.; Gonina, E.; Bentzur, J.; Hardt, M.; Recht, B.; and Talwalkar, A. 2020. A System for Massively Parallel Hyperparameter Tuning. In Dhillon, I.; Papailiopoulos, D.; and Sze, V., eds., *Proceedings of Machine Learning and Systems*, volume 2, 230–246.

Li, M.; Andersen, D. G.; Park, J. W.; Smola, A. J.; Ahmed, A.; Josifovski, V.; Long, J.; Shekita, E. J.; and Su, B.-Y. 2014. Scaling Distributed Machine Learning with the Parameter Server. In *Proceedings of the 11th USENIX Conference on Operating Systems Design and Implementation*.

Liaw, R.; Liang, E.; Nishihara, R.; Moritz, P.; Gonzalez, J. E.; and Stoica, I. 2018. Tune: A Research Platform for Distributed Model Selection and Training. *arXiv preprint arXiv:1807.05118*.

Matérn, B. 1986. *Spatial Variation*. Berlin, Germany: Springer-Verlag.

Mendes, P.; Casimiro, M.; Romano, P.; and Garlan, D. 2020. TrimTuner: Efficient Optimization of Machine Learning Jobs in the Cloud via Sub-Sampling. In *2020 28th International Symposium on Modeling, Analysis, and Simulation of Computer and Telecommunication Systems*. IEEE.

Ronneberger, O.; Fischer, P.; and Brox, T. 2015. U-Net: Convolutional Networks for Biomedical Image Segmentation. In *Medical Image Computing and Computer-Assisted Intervention – MICCAI 2015*. Springer International Publishing.

Russakovsky, O.; Deng, J.; Su, H.; Krause, J.; Satheesh, S.; Ma, S.; Huang, Z.; Karpathy, A.; Khosla, A.; Bernstein, M.; Berg, A. C.; and Fei-Fei, L. 2015. ImageNet Large Scale Visual Recognition Challenge. *International Journal of Computer Vision (IJCV)*, 115(3): 211–252.

Snoek, J.; Larochelle, H.; and P. Adams, R. 2012. Practical Bayesian Optimization of Machine Learning Algorithms. In *Proceedings of the 25th International Conference on Neural Information Processing Systems*, volume 2.

Swersky, K.; Snoek, J.; and Adams, R. P. 2014. Freeze-thaw bayesian optimization. *arXiv preprint arXiv:1406.3896*.

Valkov, L.; Jenatton, R.; Winkelmolen, F.; and Archambeau, C. 2018. A simple transfer-learning extension of Hyperband.

Wang, J.; Xu, J.; and Wang, X. 2018. Combination of Hyperband and Bayesian Optimization for Hyperparameter Optimization in Deep Learning. *arXiv preprint arXiv:1406.3896*.

Zhang, W.; Gupta, S.; Lian, X.; and Liu, J. 2016. Staleness-Aware Async-SGD for Distributed Deep Learning. In *Proceedings of the Twenty-Fifth International Joint Conference on Artificial Intelligence*, IJCAI'16, 2350–2356. AAAI Press. ISBN 9781577357704.
